# Supplementary material for: Memristive Switches in Rigid Conjugated Single-Molecule Junctions
Source: arXiv:2604.20542 source file (2026-04-22)
Supplement: Supplementary file 2 [file preamble_SI.tex]

%%%%%%%%%%%%%%%%%%%%%%%%%%%%%%%%%%%%%%%%%%%%%%%%%%%%%%%%%%%%%%%%%%%%%
%% Reference support
%%

\usepackage[
  backend=biber,
  style=chem-acs,   % chem-acs
  sorting=none,
  doi=true,
  url=false,
  isbn=false,
  eprint=false,
  articletitle=true,
  maxbibnames=999
]{biblatex}
\let\cite\supercite
\addbibresource{references_SI.bib}


% 1) Remove "In:"
\renewbibmacro{in:}{}

% 2) Remove ISSN (and hard-remove URL fields just in case)
\AtEveryBibitem{%
  \clearfield{issn}%
  \clearfield{url}%
  \clearfield{urldate}%
}

% 3) Use commas between blocks (author, title, journal, year, pages, ...)
\renewcommand*{\labelnamepunct}{\addcomma\space} % after author list
\renewcommand*{\newunitpunct}{\addcomma\space}   % between "units"
\renewcommand*{\finentrypunct}{\addperiod}       % final punctuation

% Strip " YYYY V:I" accidentally appended to journal titles (e.g. "Nature Materials 2006 5:1")
\DeclareSourcemap{
  \maps[datatype=bibtex]{
    \map{
      \step[fieldsource=journaltitle,
            match=\regexp{\s+\d{4}\s+\d+:\d+\s*$},
            replace={}]
    }
    \map{
      \step[fieldsource=journal,
            match=\regexp{\s+\d{4}\s+\d+:\d+\s*$},
            replace={}]
    }
  }
}
% Date right after journal: "Nature Materials (Dec. 2005), 5(1), ..."
\renewbibmacro*{journal+issuetitle}{%
  \usebibmacro{journal}%
  \setunit{\addspace}%
  \usebibmacro{issue+date}%
  \setunit{\addcomma\space}%
  \usebibmacro{volume+number+eid}%
  \newunit}

% Remove the number and leave only the volume
\AtEveryBibitem{\clearfield{number}}

% If you are using classical BibTeX, remove the above lines and 
% uncomment:
%\usepackage{achemso}

%%%%%%%%%%%%%%%%%%%%%%%%%%%%%%%%%%%%%%%%%%%%%%%%%%%%%%%%%%%%%%%%%%%%%
%% Graphic inclusion and scheme and chart support
%%%%%%%%%%%%%%%%%%%%%%%%%%%%%%%%%%%%%%%%%%%%%%%%%%%%%%%%%%%%%%%%%%%%%
\usepackage{graphicx}
\usepackage{xcolor}
\usepackage{float}
\newfloat{scheme}{htbp}{los}
\floatname{scheme}{Scheme}
\floatname{chart}{Chart}
\newfloat{graph}{htbp}{loh}

%%%%%%%%%%%%%%%%%%%%%%%%%%%%%%%%%%%%%%%%%%%%%%%%%%%%%%%%%%%%%%%%%%%%%
%% Common support packages
%%%%%%%%%%%%%%%%%%%%%%%%%%%%%%%%%%%%%%%%%%%%%%%%%%%%%%%%%%%%%%%%%%%%%
\usepackage{chemformula} % Formulas using \ch{}
% or
\usepackage[version = 4]{mhchem} % Formulas using \ce{}

%%%%%%%%%%%%%%%%%%%%%%%%%%%%%%%%%%%%%%%%%%%%%%%%%%%%%%%%%%%%%%%%%%%%%
%% Many journals require that sections are unnumbered: this 
%% is activated here
%%%%%%%%%%%%%%%%%%%%%%%%%%%%%%%%%%%%%%%%%%%%%%%%%%%%%%%%%%%%%%%%%%%%%
% \setcounter{secnumdepth}{-1}

%%%%%%%%%%%%%%%%%%%%%%%%%%%%%%%%%%%%%%%%%%%%%%%%%%%%%%%%%%%%%%%%%%%%%
%% Place any additional macros here.  Please use \newcommand* where
%% possible, and avoid layout-changing macros (which are not used
%% when typesetting).
%%%%%%%%%%%%%%%%%%%%%%%%%%%%%%%%%%%%%%%%%%%%%%%%%%%%%%%%%%%%%%%%%%%%%
\newcommand*\mycommand[1]{\texttt{\emph{#1}}}


% Links first
\PassOptionsToPackage{hidelinks}{hyperref}
\usepackage{hyperref}
\usepackage[nameinlink]{cleveref}
\crefname{figure}{Fig.}{Figs.}   % lowercase \cref
\Crefname{figure}{Fig.}{Figs.}   % capitalized \Cref

\usepackage{float}
\usepackage{comment}
\usepackage{siunitx}
\usepackage{svg}

\usepackage{newunicodechar}
\newunicodechar{ }{\,} % map U+2009 to a LaTeX thin space
